# Supplementary material for: Adaptive Bit Allocation for OFDM Cognitive Radio Systems with Imperfect Channel Estimation
Source: arXiv:1801.04010 source file (2019-02-08)
Supplement: Supplementary file 1 [file appendix.tex]

\section*{Appendix: \small{Derivation of NB EU variance per subcarrier ($\sigma^2_{I,k}$) (\ref{eq:var})}}
\addcontentsline{toc}{chapter}{Appendix}
%\chaptermark{Appendix}
\markboth{Appendix}{Appendix}

Here we derive the analytical expression for the NB EU variance per subcarrier ($\sigma^2_{I,k}$) after the OFDM receiver FFT. The NB EU signal is given by:
\begin{eqnarray}
I(t) & = &\sum_{l =-\infty }^{\infty}b_{l}\:p(t-lT-\xi) \:e^{j2\pi f_{c}t}, 
\end{eqnarray}
where $b_{l}$ is the $lth$ data symbol, $p(t)$ is the impulse response of the transmit filter, $T$ is the symbol period, $\xi$ is the time delay, and $f_{c}$ is the NB EU frequency deviation from the OFDM carrier frequency. As we are interested in the variance of this NB EU signal after the OFDM receiver FFT, this signal is sampled by the OFDM sampling time $T_s = \frac{1}{BW}$ resulting in
\begin{eqnarray}
I(vT_s) & = & \sum_{l =-\infty }^{\infty}b_{l}\:p(vT_s-lT-\xi)\: e^{j2\pi f_{c}vT_s}.
\label{eq:int_sam}
\end{eqnarray}
By replacing $v$ by $n+rN$, with $n$ = $0,..., N-1$ and $r$ integer, (\ref{eq:int_sam}) becomes
\begin{eqnarray}
I^r(n) & = & \sum_{l =-\infty }^{\infty}b_{l}\:p((n + rN)T_s-lT-\xi)\: e^{j2\pi f_{c}(n+rN)T_s}. 
\end{eqnarray}
The resulting signal after the OFDM receiver FFT is
\begin{eqnarray}
X^r(k) & = & \frac{1}{\sqrt{N}}\sum_{n=0}^{N-1} I^r(n) \:e^{-j\frac{2\pi kn}{N}}, \\
       & = & \frac{1}{\sqrt{N}}\sum_{n=0}^{N-1} \sum_{l =-\infty }^{\infty}b_{l}\: p((n + rN)T_s-lT-\xi)\: e^{j2\pi f_{c}(n+rN)T_s} \: e^{-j\frac{2\pi kn}{N}}.
\end{eqnarray}
Finally, the variance of NB EU signal after the OFDM receiver FFT can be written as
\begin{eqnarray}
(\sigma^{r}_{I,k})^2 & = & \mathbb E\left \{ X^r(k) X^{*r}(k) \right \} \nonumber \\
% & = & \frac{1}{N}\sum_{n=0}^{N-1}\sum_{n'=0}^{N-1} \sum_{l =-\infty }^{\infty} \sum_{l' =-\infty }^{\infty} \mathbb E \{b_l b^*_{l'}\} \: p((n + rN)T_s-lT-\xi) \: p((n + rN)T_s-lT-\xi) \nonumber \\
% & & e^{j2\pi f_{c}(n+rN)T_s} \: e^{-j2\pi f_{c}(n'+rN)T_s} \: e^{-j\frac{2\pi kn}{N}} \: e^{j\frac{2\pi kn'}{N}}, \\
 & = & \frac{\sigma_b^2}{N} \sum_{n=0}^{N-1}\sum_{n'=0}^{N-1} \sum_{l =-\infty }^{\infty} p((n + rN)T_s-lT-\xi) \: p((n + rN)T_s-lT-\xi) \nonumber \\
 & & e^{j2\pi f_{c}(n-n')T_s} \: e^{-j\frac{2\pi k}{N}(n-n')}, \nonumber
\end{eqnarray}
where $\mathbb E\{.\}$ denotes the statistical expectation operator, and $\sigma_b^2$ = $\mathbb E\{b_l b^*_l\}$. By averaging over the number of OFDM symbols $R$, the NB EU variance per subcarrier can be finally expressed as
\begin{eqnarray}
 \sigma^2_{I,k} & = & \lim_{R \rightarrow \infty} \frac{1}{R} \frac{\sigma_b^2}{N} \sum_{r = 0}^{R-1} \sum_{n=0}^{N-1}\sum_{n'=0}^{N-1} \sum_{l =-\infty }^{\infty} p((n + rN)T_s-lT-\xi) \: p((n + rN)T_s-lT-\xi) \nonumber \\
 & & e^{j2\pi f_{c}(n-n')T_s} \: e^{-j\frac{2\pi k}{N}(n-n')}.
\end{eqnarray}
